# Supplementary material for: $\mbox{Bi}_{1}\mbox{Te}_{1}$: a dual topological insulator
Source: arXiv:1604.08886 source file (2016-04-29)
Supplement: Supplementary file 1 [file SupplementaryMaterial.pdf]

# Supplementary material to: $\mathbf{Bi_1Te_1}$ : a dual topological insulator

Markus Eschbach*, Martin Lanius*, Chengwang Niu*, Ewa Młyńczak, Pika Gospodarič, Jens Kellner, Peter Schüffelgen, Mathias Gehlmann, Sven Döring, Elmar Neumann, Martina Luysberg, Bernhard Holländer, Gregor Mussler, Lukasz Plucinski†, Markus Morgenstern, Detlev Grützmacher, Gustav Bihlmayer, Stefan Blügel, and C.M. Schneider

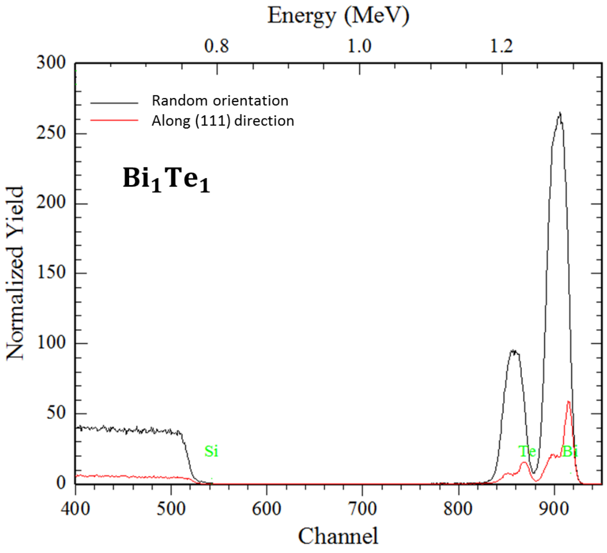


Figure 1: Rutherford backscattering spectrum of a 50 nm thick $Bi_1Te_1$ film for the accurate determination of stoichiometry.

## I. CHARACTERIZATION

*Rutherford Back Scattering.*

The sample was analyzed by Rutherford backscattering spectrometry / ion channeling using 1.4 MeV He+ ions and a backscattering angle of 170 degrees. Fig. 1 shows the corresponding random (black) and (111)-channeling (red) spectra. The areal coverage of Te and Bi was determined by individual peak integration, yielding a Bi : Te ratio of 1:1 within the experimental accuracy which is estimated to be 1%. The channeling spectrum exhibits clear surface peaks of Te and Bi and the minimum yield of about 7% determined behind the surface peak confirms the single crystalline, epitaxial growth on the Si(111) substrate with good crystalline quality.

*2D Reciprocal space maps.*

Figure 2 depicts two-dimensional reciprocal space maps around the (1,0,-1,20) reflection for $Bi_2Te_3$ (left) and the (1,0,-1,16) reflection for $Bi_1Te_1$ (right). From this, the in-plane and out-of-plane lattice constants, denoted in the figure, could be obtained.

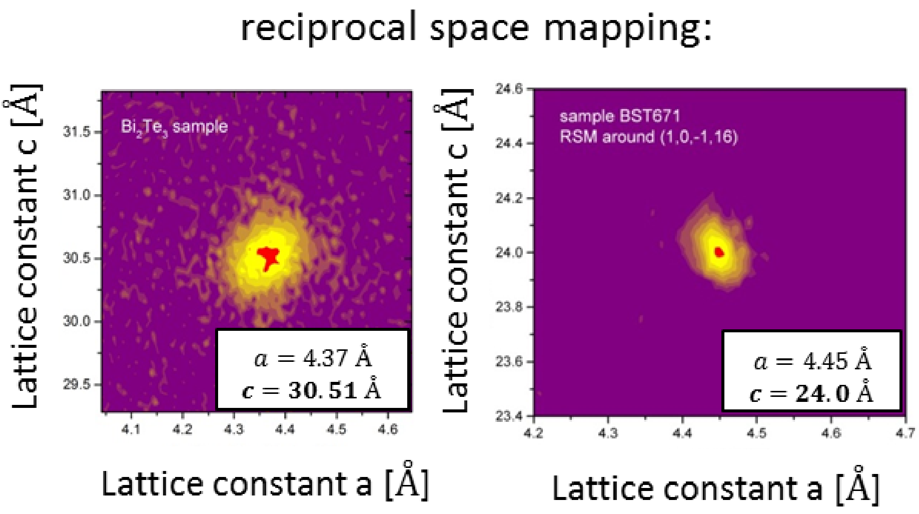


Figure 2: 2D reciprocal space maps obtained from X-ray diffraction using $h\nu = 8047.7\,\mathrm{eV}$ of a $Bi_2Te_3$(left) and a $Bi_1Te_1$ (right) film.

## II. SURFACE CHEMISTRY AND THE INFLUENCE OF SPUTTERING ON THE SURFACE TERMINATION

Thin films of $Bi_1Te_1$ were either measured 'as grown' or as 'sputtered' samples, which were altered by gentle Ar sputtering with 750 eV ions and subsequent annealing up to 200°C for 15 min. Since the sputtering yield ratio between Te and Bi is $^{5.7}/_{3.3} \approx 1.7$ [1], a Te deficiency results in favorably Bi-rich, i.e., Bi BL terminated surfaces. In contrast, the 'as grown' samples are, due to the growth mode, expected to exhibit Bi-poor, i.e., QL terminated surfaces. Thus, it turns out that the Bi BL density on the surface can be significantly enhanced by Ar bombardment and annealing due to differences in sputtering yields of Te and Bi, resulting in differences in the surface electronic structure of these Bi-poor and Bi-rich surfaces. In the following this will be investigated using X-ray spectroscopy (XPS) and angle-resolved photoemission (ARPES). XPS reveals that Bi exhibits different binding energies in QLs and BLs, which can be used for identification of the near-surface density of QLs and BLs.

*X-ray photoelectron spectroscopy.*

For x-ray photoelectron spectroscopy of the shallow Bi 5d and Te 4d core levels with ($h\nu = 100\,\mathrm{eV}$) as well as for the spin-resolved ARPES measurements ($h\nu = 22\,\mathrm{eV}$) we used

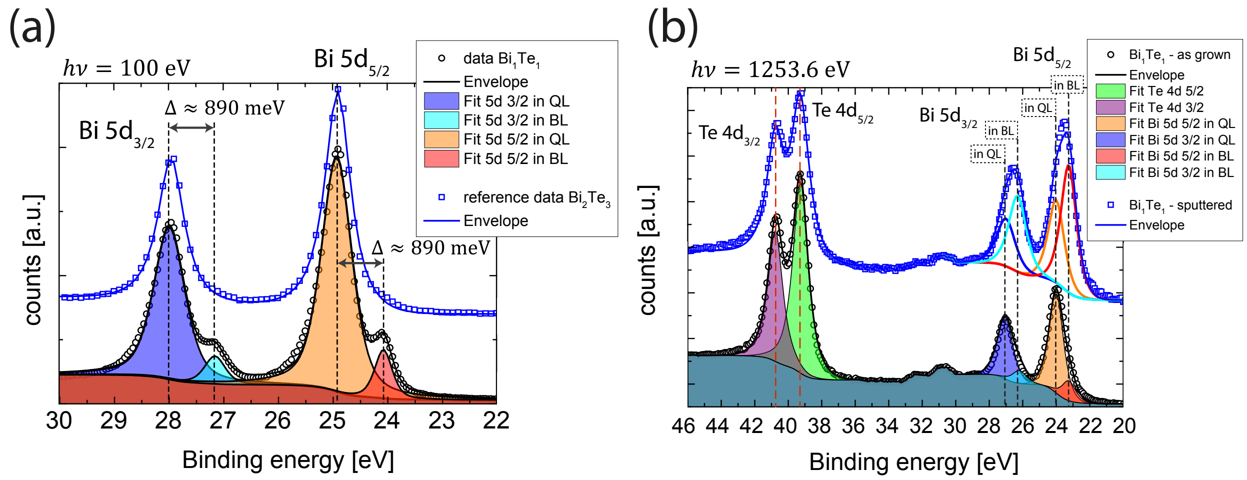


Figure 3: (a) High-resolution XPS spectra of the Bi 5d shallow core level for both $Bi_2Te_3$ and $Bi_1Te_1$ thin films taken with $h\nu = 100\,\text{eV}$ at BL5. Individual components of the peaks are determined and highlighted separately. (b) In situ laboratory-based XPS study on $Bi_1Te_1$ after growth and after sputtering using $h\nu = 1253.6\,\text{eV}$ at Te 4d and Bi 5d core levels. The Bi : Te ratio can be determined by extracting the peak areas.

a Scienta SES-2002 spectrometer and a Focus SPLEED polarimeter at beamline BL5 of the DELTA synchrotron in Dortmund at room temperature, resulting in an energy resolution of $\approx 100\,\text{meV}$ [2]. Here, clean sample surfaces are prepared by sputtering and annealing after sample transfer through air, which resulted in Bi-rich sample surfaces. Additionally, a lab-based XPS study was performed before and after sputtering and annealing of $Bi_1Te_1$ in order to quantify the change in surface chemistry. Therefore, we used a standard non-monochromatized Mg $K_\alpha$ X-ray tube and an Omicron spectrometer resulting in an energy resolution of $\approx 700\,\text{meV}$.

Figure 3(a) shows high-resolution XPS spectra on the Bi 5d shallow core level of a $Bi_2Te_3$ reference film (blue symbols), and a sputtered $Bi_1Te_1$ film (black symbols). The peak splitting in the $Bi_1Te_1$ sample by $\Delta \approx 890\,\text{meV}$ in each of the spin-orbit split doublets, which is not present in the $Bi_2Te_3$ reference sample, proves the existence of the Bi BL close to the surface. It indicates that Bi exists in two distinct chemical environments. Comparison with the literature data confirms that the high-binding energy component originates from Bi bound in a bilayer, while the low-binding energy component is related to Bi located inside a quintuple layer [3, 4].

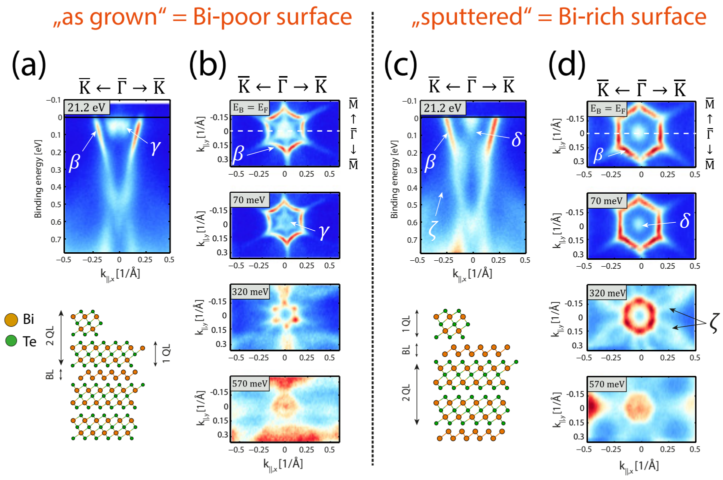


Figure 4: Effect of sputtering and annealing on the surface electronic structure of $Bi_1Te_1$. (a) [c] $E_B$ vs. $k_{||}$ spectra along $\overline{\Gamma K}$ direction of the as grown $Bi_1Te_1$ surface [after sputtering and annealing], recorded using $h\nu = 21.2\,eV$ at low temperatures. A simplified scheme of the surface crystal structure is shown below (orange = Bi atoms; green = Te atoms). (b) [d] Corresponding constant energy contours at indicated binding energies.

In order to show that sputtering removes Te more efficiently and, thus, produces Bi-rich surfaces, Fig. 3(b) depicts the Bi and Te core level spectra of $Bi_1Te_1$ immediately after growth and after subsequent sputtering and annealing (black symbols = $Bi_1Te_1$ as grown; blue symbols = $Bi_1Te_1$ sputtered). As compared to the results presented in Fig. 3(a), the energy resolution is worse, since a non-monochromatized Mg $K_\alpha$ source is used, and, consequently, the features are broadened. Nevertheless, we fitted the peaks with two components for Te 4d and four components for Bi 5d, using the splitting as defined from Fig. 3(a). The total Bi signal with respect to the Te signal has significantly increased upon sputtering. Using the same fitting parameters for both curves and constraining spin-orbit coupling induced peak ratios of 3d levels and the peak positions to the values deduced from Fig. 3(a), we can extract the Bi : Te ratios as well as the Bi QL : BL ratios from the filled peak areas, respectively. The total Bi signal has increased by a factor of 2.0 and the QL : BL ratio has dramatically decreased from 5.2 to 0.7 upon sputtering. This effect also appears directly as an energetic shift of the blue Bi peak with respect to be black one, while the Te peaks are not shifted at all. Thus, indeed, the amount of Bi BL in $Bi_1Te_1$ can be dramatically increased by sputtering and annealing.

*Influence of sputtering seen by ARPES.*

In order to perform spin-ARPES measurements at the synchrotron-based beamline at DELTA, samples needed to be prepared by sputtering and annealing. Therefore, we investigate and discuss the effect of sputtering on the electronic structure and the results are summarized in Fig. 4. Here, panels (a) and (c) show near-Fermi level $E_\mathrm{B}$ vs. $k_{||}$ spectra along $\overline{\Gamma\mathrm{K}}$ direction for the as grown, i.e. Bi-poor, surface and the sputtered, i.e., Bi-rich, surface of a $Bi_1Te_1$ thin film, respectively. Panels (b) and (d) display corresponding $k_{||}^x$ vs. $k_{||}^y$ constant energy contours at $E_\mathrm{B} = E_\mathrm{F}$, 70 meV, 320 meV and 570 meV.

First of all, the changes in the crystal quality and ARPES spectra are not dramatic and the general structure remains unaltered. Upon sputtering, i.e. producing a Bi-rich surface (see Fig. 3), the most prominent $\beta$ band does not change at all (Figs. 4(a) and (c)) but the material gets even further n-doped which can be seen by a slightly larger area within the $\beta$ band in the Fermi surface. The strongest difference between the as grown and the sputtered $Bi_1Te_1$ samples are the vanishing parabolic electron-like $\gamma$ bands, having six-fold symmetric shape in the constant energy cut closely below the Fermi level, and the appearance of the hole-like, more linearly dispersing $\delta$ and $\zeta$ bands which have a circular shape close to the Fermi surface and appear as strong six-fold symmetric bands around 320 meV below Fermi level.

We interpret the $\gamma$ bands as being created by domains of 2 QL termination, whereas the latter $\delta$ and $\zeta$ states originate from Bi BLs, as the good agreement to the calculations in Fig. 2 of the main article indicates, respectively. Hence, in $Bi_1Te_1$ it is possible to modify the electronic structure by manipulating the surface termination by sputtering. In other words, one is able to "switch" on and off certain bands, while other features as well as the general structure remains constant.

## III. SUPERPOSITION OF MULTIPLE SURFACE TERMINATIONS

As we have seen in Fig. 2 of the main article, $Bi_1Te_1$ due to its unit cell and the layered nature can naturally exhibit three different surface terminations, which we can not distinguish between in our ARPES measurements since we are lacking the lateral resolution. The ARPES spectra in Fig. 4 of the main article do not resemble the band gap close to the Fermi level that is predicted to open up along the $\overline{\Gamma\mathrm{K}}$ direction. Since there is no mirror

symmetry protecting a crossing of the bands along this direction, a band gap should open up, as one can see in the DFT surface calculations in Fig. 2 for the 1QL terminated surface. However, already the surface terminated by 2QLs will exhibit additional non-crossing states making the situation even more complicated. Therefore, it is very likely that our spatially averaging technique will measure a superposition of differently terminated surfaces which can easily explain the not observed band gap. Figure 5 shows the magnified HR ARPES spectrum from Fig. 4 and the calculated spectra from Fig. 2 for both the 1QL and 2QL case, for comparison.

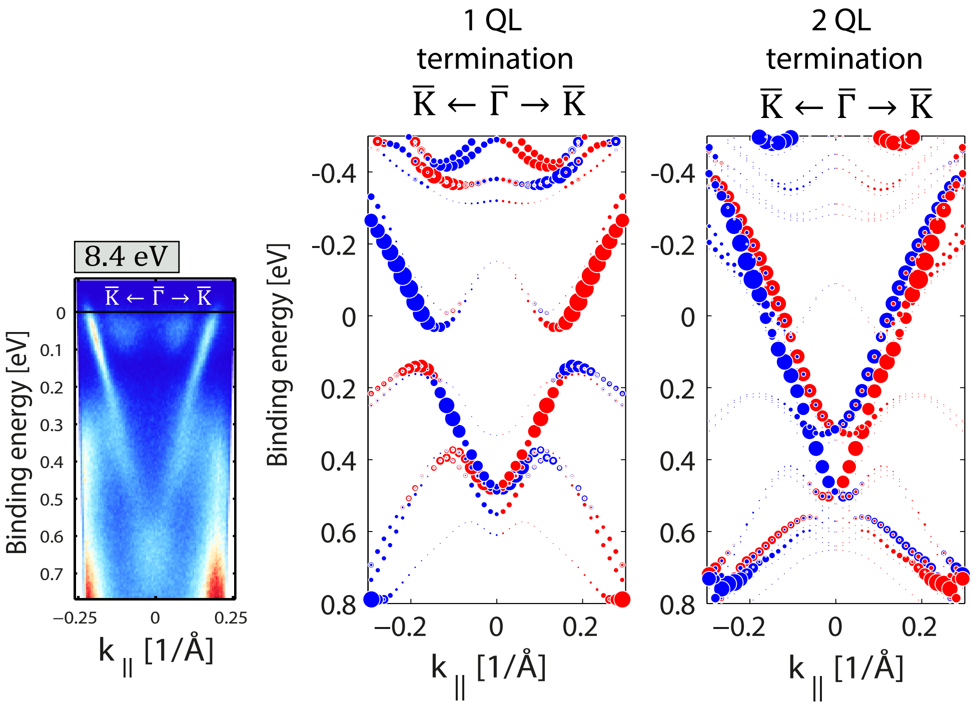


Figure 5: Comparison of the HR ARPES measurement obtained using $h\nu = 8.4\,\mathrm{eV}$ (from main Fig. 4) and the magnified calculated spectra (from main Fig. 2) along $\overline{\Gamma\mathrm{K}}$ direction close to the Fermi level.

[1] N. P. Laboratory, `Databaseofsputteringyields`.
URL `http://www.npl.co.uk/science-technology/surface-and-nanoanalysis/services/sputter-yield-values`

[2] L. Plucinski, A. Oelsner, F. Matthes, C. Schneider, Journal of Electron Spectroscopy and Related Phenomena 181 (2010) 215–219.

[3] T. Valla, H. Ji, L. Schoop, A. Weber, Z.-H. Pan, J. T. Sadowski, E. Vescovo, A. V. Fedorov, A. N. Caruso, Q. D. Gibson, L. Müchler, C. Felser, R. Cava, Topological semimetal in a $Bi - Bi_2Se_3$ infinitely adaptive superlattice phase, Physical Review B 86 (2012) 241101.

[4] Q. D. Gibson, L. M. Schoop, A. P. Weber, H. Ji, S. Nadj-Perge, I. K. Drozdov, H. Beidenkopf, J. T. Sadowski, A. Fedorov, A. Yazdani, T. Valla, R. J. Cava, Termination-dependent topological surface states of the natural superlattice phase $Bi_4Se_3$, Physical Review B 88 (2013) 081108.
